# Supplementary material for: RVHyper: A Runtime Verification Tool for Temporal Hyperproperties
Source: arXiv:1906.00798 source file (2019-05-31)
Supplement: Supplementary file 1 [file appendix.tex]

\section{Proofs}

\begin{lemma} \label{thm:exists-2-dominance}
	Given an $\exists^2$ HyperLTL formula $\varphi$ over trace variables $\pathvars := \{\pi_1, \ldots, \pi_n\}$ and two traces $t,t' \in \traces$, the following holds: $t$ dominates $t'$ if and only if
	\[
	\lang(\monitor_\varphi[t'/\pi_1]) \subseteq \lang(\monitor_\varphi[t/\pi_1]) \wedge \lang(\monitor_\varphi[t'/\pi_2]) \subseteq \lang(\monitor_\varphi[t/\pi_2])
	\]
\end{lemma}
\begin{proof}
  Assume for the sake of contradiction that (a) $t$ dominates $t'$ and w.l.o.g. (b) $\lang(\monitor_\varphi[t'/\pi_1]) \nsubseteq \lang(\monitor_\varphi[t/\pi_1])$.
  Thus, by definition of subset, there exists a trace $\tilde{t}$ with $\tilde{t} \in \lang(\monitor_\varphi[t'/\pi_1])$ and $\tilde{t} \not \in \lang(\monitor_\varphi[t/\pi_1])$.
  Hence, $\pathassign = \set{\pi_1 \mapsto t', \pi_2 \mapsto \tilde{t}}$ is a valid trace assignment, whereas $\pathassign' = \set{\pi_1 \mapsto t, \pi_2 \mapsto \tilde{t}}$ is not.
  On the other hand, from (a) the following holds by Definition~\ref{def_dominance}: $\forall T'$ with $\set{t} \subseteq T'$ it holds that $T' \in \lang(\varphi) \Leftrightarrow T' \cup \{t'\} \in \lang(\varphi)$.
  We choose $T'$ as $\{t,\tilde{t}\}$, which is a contradiction to the equivalence since we know from (a) that $\pathassign$ is a valid trace assignment, but $\pathassign'$ is not a valid trace assignment.

  For the other direction, assume that $\lang(\monitor_\varphi[t'/\pi_1]) \subseteq \lang(\monitor_\varphi[t/\pi_1])$ and $\lang(\monitor_\varphi[t'/\pi_2]) \subseteq \lang(\monitor_\varphi[t/\pi_2])$.
  Let $T'$ be arbitrary such that $\set{t} \subseteq T'$.
  We distinguish two cases:
  \begin{itemize}
  	\item
      Case $T' \cup \set{t'} \in \lang(\varphi)$, then (a) $T' \subseteq \lang(M_\varphi[t'/\pi_1]) \subseteq \lang(M_\varphi[t/\pi_1])$ and (b) $T' \subseteq \lang(M_\varphi[t'/\pi_2]) \subseteq \lang(M_\varphi[t/\pi_2])$.
      By Lemma~\ref{thm:language-inclusion-by-iteration} and $T' \cup \set{t'} \in \lang(\varphi)$, it follows that $T' \in \lang(\varphi)$.
  \item
      Case $T' \cup \set{t'} \notin \lang(\varphi)$, then $T' \notin \lang(\varphi)$.
  \end{itemize}
\end{proof}

\begin{proof}[of Theorem~\ref{thm:forall-exists-dominance}]
  The $\Rightarrow$ direction is the same as in proofs of Theorem~\ref{dominating} and Lemma~\ref{thm:exists-2-dominance}.
  
  For the other direction, assume that that (a) $\lang(\monitor_\varphi[t/\pi]) \subseteq \lang(\monitor_\varphi[t'/\pi])$ and (b) $\lang(\monitor_\varphi[t'/\pi']) \subseteq \lang(\monitor_\varphi[t/\pi'])$.
  Let $T'$ be arbitrary such that $\set{t} \subseteq T'$.
  We distinguish two cases:
  \begin{itemize}
    \item
      Case $T' \in \lang(\varphi)$, then for all $t_1 \in T'$ there is a $t_2 \in T'$ such that $\pathassignfin = \set{\pi \mapsto t_1, \pi' \mapsto t_2} \models_\emptyset \psi$.
      Especially, for $t$, there is a corresponding trace $t^*$ such that $\set{\pi \mapsto t, \pi' \mapsto t^*} \models_\emptyset \psi$, thus $t^* \in \lang(\monitor_\varphi[t/\pi])$.
      From (a) it follows that $t^* \in \lang(\monitor_\varphi[t'/\pi])$.
      Hence, $\set{\pi \mapsto t', \pi' \mapsto t^*} \models_\emptyset \psi$ and thereby $T' \cup \set{t'} \in \lang(\varphi)$.
    \item
      Case $T' \cup \set{t'} \in \lang(\varphi)$, then for all $t_1 \in T' \cup \set{t'}$ there is a $t_2 \in T' \cup \set{t'}$ such that $\set{\pi \mapsto t_1, \pi' \mapsto t_2} \models_\emptyset \psi$.
      Assume for the sake of contradiction there is a $t_1 \in T'$ such that there is no $t_2 \in T'$ with $\set{\pi \mapsto t_1, \pi' \mapsto t_2} \models_\emptyset \psi$.
      It follows that $\set{\pi \mapsto t_1, \pi' \mapsto t'} \models_\emptyset \psi$, i.e., $t_1 \in \lang(\monitor_\varphi[t'/\pi'])$.
      From (b) it follows that $t_1 \in \lang(\monitor_\varphi[t/\pi'])$, leading to the contradiction that $\set{\pi \mapsto t_1, \pi' \mapsto t} \models_\emptyset \psi$ and $t \in T'$.
      Hence, $T' \in \lang(\varphi)$.
  \end{itemize}
\end{proof}

\begin{proof}[of Lemma~\ref{thm:hyperltl-body-to-ltl}]
	Assume that there is a trace assignment $A$ over trace variables $\pathvars$ such that $A \models_\emptyset \psi$.
	We define $w \subseteq \Sigma_\pathvars^\omega$ such that $x_\pi \in w[i]$ if, and only if, $x \in A(\pi)[i]$ for all $i \geq 0$, $x \in \ap$, and $\pi \in \pathvars$.
	An induction over $\psi$ shows that $w \models_\ltl \psi$.
	
	Assume $\psi$ is satisfiable for $\models_\ltl$, i.e., there exists a $w \subseteq \Sigma^\omega_\pathvars$, such that $w \models_\ltl \psi$.
	We construct an assignment $A$ in the following manner: Let $\pi \in \pathvars$ be arbitrary.
	We map $\pi$ to the trace $t$ obtained by projecting the corresponding $p_\pi \in \Sigma_\pathvars$, i.e., $\forall i \geq 0 \ldot t[i] = \#_\pi(w[i])$.
	\qed
\end{proof}

\begin{proof}[of Lemma~\ref{thm:forall-good-empty}]
	If $\psi \equiv \true$ then $\lang(\varphi) = \powerset(\Sigma^\omega)$ and $\good(\lang(\varphi)) = \powerset^*(\Sigma^*)$.
	Assume for contradiction that $\psi \not\equiv \true$ and $\good(\lang(\varphi)) \neq \emptyset$, i.e., there is a finite set $U \subseteq \Sigma^*$ that is a good prefix set of $\varphi$.
	Since $\psi \neq \true$, there is at least one infinite trace $\sigma$ with $\sigma \nmodels \psi$.
	We translate this trace to a set of infinite traces $W$ where $W \nmodels \varphi$ using Lemma~\ref{thm:hyperltl-body-to-ltl}.
	Further, for all $V \in \powerset(\Sigma^*)$ with $U \pref V$, it holds that $W \subseteq V$, hence, $V \notin \lang(\varphi)$ violating the assumption that $U \in \good(\lang(\varphi))$.
	\qed
\end{proof}

%\begin{theorem}
%	Algorithm~\ref{alg_minimization} preserves the minimal trace set $T$, i.e., for all $t \in T$ it holds that $t$ is not $(T \setminus \set{t},\varphi)$-redundant.
%\end{theorem}
\begin{proof}[of Theorem~\ref{alg}]
	By induction on $T \setminus \set{t}$ and Theorem~\ref{dominating}.
	\qed
\end{proof}

\section{Tables}
We extended Table~\ref{formulaanalysis} with $\hyperltl$ formulas used in a case study in~\cite{conf/cav/FinkbeinerRS15} to verify versions of the bakery protocol (symm1 - symm2) and error resisting codes (Ham).
\begin{table}[]
	\centering
	\caption{Formula Analysis for universally quantified hyperproperties studied in the literature. Each property has been checked in under $1 s$.}
	\label{formulaanalysis-extended}
	\begin{tabular}{ll|l|l|l|}
		\cline{3-5}
		&                                                                                                                                                                                                                                                                                                                                                                                                                                                                    & symm & trans & refl \\ \hline
		\multicolumn{1}{|l|}{ObsDet1}     & $\forall \pi. \forall \pi'.\; \G (I_{\pi} = I_{\pi'}) \rightarrow \G (O_{\pi} = O_{\pi'})$                                                                                                                                                                                                                                                                                                                                                             &  \cmark    &    \xmark   &  \cmark    \\ \hline
		\multicolumn{1}{|l|}{ObsDet2}     & $\forall \pi. \forall \pi'.\; (I_{\pi} = I_{\pi'}) \rightarrow \G (O_{\pi} = O_{\pi'})$                                                                                                                                                                                                                                                                                                                                                                &  \cmark    &    \xmark   &  \cmark      \\ \hline
		\multicolumn{1}{|l|}{ObsDet3}     & $\forall \pi. \forall \pi'. O_\pi = O_\pi' \W I_\pi \neq I_\pi'$                                                                                                                                                                                                                                                                                                                                                                                                   &  \cmark    &    \xmark   &  \cmark      \\ \hline
		\multicolumn{1}{|l|}{QuantNoninf} & $\forall \pi_0 \ldots \forall \pi_{c}.~\neg ((\bigwedge_i I_{\pi_i} = I_{\pi_0}) \wedge \bigwedge_{i \neq j} O_{\pi_i} \neq O_{\pi_j})$                                                                                                                                                                                                                                                                                                                            &  \cmark    &    \xmark   &  \cmark      \\ \hline
		\multicolumn{1}{|l|}{Ham}         & \begin{tabular}[c]{@{}l@{}}$\forall \pi.\; \forall \pi'.\; F (\bigvee_{i\in I} \neg (i_\pi \leftrightarrow i_{\pi'})) \rightarrow \neg \mathit{Ham}_O(d-1,\pi,\pi')$\\ $\mathit{Ham_O}\coloneqq \mathit{Ham_O}(-1,\pi,\pi') = \mathit{false}$ and\\ $\mathit{Ham_O}(d,\pi,\pi') = (\bigwedge_{o\in O} o_\pi \leftrightarrow o_{\pi'})$ \\       $\W (\bigvee_{o\in O} \neg (o_\pi \leftrightarrow o_{\pi'}) \wedge \X\;\mathit{Ham_O}(d-1,\pi,\pi'))$\end{tabular} &  \cmark    &    \xmark   &  \cmark      \\ \hline
		\multicolumn{1}{|l|}{Symm1}       & \begin{tabular}[c]{@{}l@{}}$\forall \pi. \forall \pi'. \G (\mathit{sym}(\mathit{sel}_\pi, \mathit{sel}_{\pi'}) \wedge pause_\pi = pause_{\pi'})$\\ $\rightarrow \G(\mathit{pc}(0)_\pi = \mathit{pc}(1)_{\pi'} \wedge \mathit{pc}_\pi = \mathit{pc}(0)_{\pi'})$\end{tabular}                                                                                                                                                                                        &  \xmark    &    \xmark   &  \cmark      \\ \hline
		\multicolumn{1}{|l|}{Symm2}       & \begin{tabular}[c]{@{}l@{}}$\forall \pi. \forall \pi'. \G (\mathit{sym}(\mathit{sel}_\pi, \mathit{sel}_{\pi'}) \wedge pause_\pi = pause_{\pi'}$\\ $\wedge \mathit{sel}_\pi < 3 \wedge \mathit{sel}_{\pi'} < 3)$\\ $\rightarrow \G(\mathit{pc}(0)_\pi = \mathit{pc}(1)_{\pi'} \wedge \mathit{pc}_\pi = \mathit{pc}(0)_{\pi'})$\end{tabular}                                                                                                                         &  \xmark    &    \xmark   &  \xmark      \\ \hline
		\multicolumn{1}{|l|}{Symm3}       & \begin{tabular}[c]{@{}l@{}}$\forall \pi. \forall \pi'. \G (\mathit{sym}(\mathit{sel}_\pi, \mathit{sel}_{\pi'}) \wedge pause_\pi = pause_{\pi'})$\\ $\wedge \mathit{sel}_\pi < 3 \wedge \mathit{sel}_{\pi'} < 3 \wedge \mathit{sym}(\mathit{symbreak}_\pi,\mathit{symbreak}_{\pi'})$\\ $\rightarrow \G(\mathit{pc}(0)_\pi = \mathit{pc}(1)_{\pi'} \wedge \mathit{pc}_\pi = \mathit{pc}(0)_{\pi'})$\end{tabular}                                                     &  \xmark    &    \xmark   &  \xmark    \\ \hline
		
		\multicolumn{1}{|l|}{ConfMan} &\begin{tabular}[c]{@{}l@{}}$\forall \pi \forall \pi' \ldot \big((\neg pc_\pi \wedge pc_{\pi'}) \rightarrow \X\G (s_\pi \rightarrow \X v_{\pi'})\big)$\\ $\wedge \big((pc_{\pi} \wedge pc_{\pi'}) \rightarrow \X\G (v_\pi \leftrightarrow v_\pi')\big)$\end{tabular} &  \xmark    &    \xmark   &  \xmark \\ \hline
		
		\multicolumn{1}{|l|}{EQ} &\begin{tabular}[c]{@{}l@{}}$\forall \pi. \forall \pi' \ldot \G (a_\pi \leftrightarrow a_{\pi'})$\end{tabular} &  \cmark    &    \cmark   &  \cmark \\ \hline
	\end{tabular}
\end{table}
